# Supplementary material for: Accounting for Work Zone Disruptions in Traffic Flow Forecasting
Source: arXiv:2407.11407 source file (2024-07-16)
Supplement: Supplementary file 1 [file Appendix.tex]

%\section*{Appendix}
%Summary of notations used in this paper.
\begin{table}[htbp]
\centering
{Appendix - Frequently-used mathematical notations.}
%\label{table 1}
\small
\begin{tabular}{|p{3.2em}|p{20em}|}
\hline
Notation & Description\\
\hline
$G$ & a directed sensor network \\
$V$ & road segments/ sensors \\
$E$ & road distance for each pairs of sensors \\
$A/A_{v_iv_j}$& weighted adjacency matrix of $G$\\
$X/X_{v_it_j}$& a feature map \\
$X_T$ & traffic speeds over past $P$ time steps\\
$U$ & matrix  of  eigenvectors  ordered  by eigenvalue \\
$D/L$ & undirected degree matrix / Laplacian matrix \\
$g_\theta / *$ & a learnable convolution kernel \\
\hline
$N / n$ & number of road segments / n$^{\mathrm{th}}$ road segment \\
$T / k$ & length of historical time series / k$^{\mathrm{th}}$ time step \\
$H / h$ & number of time steps for training / h$^{\mathrm{th}}$ time step\\
$P / p$ & number of time steps for predicting / p$^{\mathrm{th}}$ time step\\
$v_i$ & traffic speeds measured in road segment $i$\\
$t_j$ & traffic speeds measured at time $j$\\

\hline
$\lambda$ & a hyper-parameter in construction work feature map\\
$\odot$ & Hadamard product \\
$W_s / W_c$ & learning parameters  \\
\hline
$U$ & the matrix of eigenvectors ordered by eigenvalues\\
$\Lambda$ & the diagonal matrix of eigenvalues \\
$\ast$     & graph convolution operation \\
$\lambda_{max}$ & spectral radius \\
$\theta$ & the vector of Chebyshev coefficient \\
$\sigma$    &   an activation function \\
\hline
\end{tabular}
\end{table}
